# Supplementary material for: A limiter-based approach to construct high-order fully-discrete entropy stable explicit DG schemes for hyperbolic conservation laws
Source: arXiv:2603.27478 source file (2026-11-12)
Supplement: Supplementary file 1 [file ex_supplement.tex]

% SIAM Supplemental File Template
\documentclass[review,supplement,hidelinks,onefignum,onetabnum]{siamart220329}

\input{ex_shared}
\usepackage{subfigure}

\externaldocument[][nocite]{ex_article}

% Optional PDF information
\ifpdf
\hypersetup{
  pdftitle={Supplementary materials: A globally divergence-free entropy stable nodal DG method for conservative ideal MHD equations},
  pdfauthor={?}
}
\fi

\begin{document}

\maketitle

%In this attachment we give 

\section{Entropy conservative flux and entropy stable flux}\label{app}

\subsection{Entropy conservative flux}

For the MHD equations, Chandrashekar and Klingengberg \cite{chandrashekar2016entropy} suggested the following entropy conservative flux:
\begin{align*}
\mathbf{F}_{1}^{S}&=\hat{\rho}\bar{u}_x,
\\
\mathbf{F}_{2}^{S}&=\frac{\bar{\rho}}{2\bar{\beta}}+\bar{u}_x\mathbf{F}_{1}^{S}+\frac{1}{2}\overline{\left\| \mathbf{B} \right\| ^2}-\bar{B}_x\bar{B}_x,
\\
\mathbf{F}_{3}^{S}&=\bar{u}_y\mathbf{F}_{1}^{S}-\bar{B}_x\bar{B}_y,
\\
\mathbf{F}_{4}^{S}&=\bar{u}_z\mathbf{F}_{1}^{S}-\bar{B}_x\bar{B}_z,
\\
\mathbf{F}_{6}^{S}&=0,
\\
\mathbf{F}_{7}^{S}&=\frac{1}{\bar{\beta}}\left( \overline{\beta u_x}\bar{B}_y-\overline{\beta u_y}\bar{B}_x \right), 
\\
\mathbf{F}_{8}^{S}&=\frac{1}{\bar{\beta}}\left( \overline{\beta u_x}\bar{B}_z-\overline{\beta u_z}\bar{B}_x \right),
\\
\mathbf{F}_{5}^{S}&=\frac{1}{2}\left[ \frac{1}{\left( \gamma -1 \right) \hat{\beta}}-\overline{\left\| \mathbf{u} \right\| ^2} \right] \mathbf{F}_{1}^{S}+\bar{u}_x\mathbf{F}_{2}^{S}+\bar{u}_y\mathbf{F}_{3}^{S}+\bar{u}_z\mathbf{F}_{4}^{S}
\\
&+\bar{B}_x\mathbf{F}_{6}^{S}+\bar{B}_y\mathbf{F}_{7}^{S}+\bar{B}_z\mathbf{F}_{8}^{S}-\frac{1}{2}\bar{u}_x\overline{\left\| \mathbf{B} \right\| ^2}+\left( \bar{u}_x\bar{B}_x+\bar{u}_y\bar{B}_y+\bar{u}_z\bar{B}_z \right) \bar{B}_x, 
\end{align*}
where $\overline{(a,b)}=(a+b)/2$ is the arithmetic average, and $\hat{(\cdot)}$ is the logarithmic average of two strictly positive quantities as
$$ \hat\alpha = \frac{\alpha_r-\alpha_l}{\ln\alpha_r-\ln\alpha_l}. $$
The formula of $\mathbf G^S$ is similar.

\subsection{Entropy stable flux}

For entropy stable fluxes, it is well known that the Godunov
flux based on exact Riemann solvers is by definition entropy stable. Meanwhile, many approximate Riemann solvers, such as the HLL
or Lax–Friedrichs fluxes are also entropy stable if the estimates of left and right local wave speed $S_L,\ S_R$ satisfy $S_L\le S_L^{real},\ S_R\ge S_R^{real}$, where $S_{L,R}^{real}$ are the real minimal and maximal wave speed of the Riemann problem at the interface \cite{chen2017entropy}. In particular, the HLL flux is given by
\begin{equation*}
\hat{\mathbf{F}}^{HLL}\left( \mathbf{U}_L,\mathbf{U}_R \right) =\left\{\begin{aligned}
	&\mathbf{F}(\mathbf{U}_L),\quad S_L\ge 0,\\
	&\frac{S_R\mathbf{F}_L-S_L\mathbf{F}_R+S_RS_L\left( \mathbf{U}_R-\mathbf{U}_L \right)}{S_R-S_L},\quad S_L<0<S_R,\\
	&\mathbf{F}(\mathbf{U}_R),\quad S_R\le 0,\\
\end{aligned}\right.
\end{equation*}
If we denote the non-positive part of $S_L$ by $\mathcal S_L=\min\{S_L,0\}$, and the non-negative part of $S_R$ by $\mathcal S_R=\max\{S_R,0\}$, then the HLL flux can be written by
\begin{equation}\label{eq:HLL} \hat{\mathbf F}^{HLL}(\mathbf U_L,\mathbf U_R) = \frac{\mathcal S_R\mathbf F_L-\mathcal S_L\mathbf F_R+\mathcal S_R\mathcal S_L(\mathbf U_R-\mathbf U_L)}{\mathcal S_R-\mathcal S_L}.
\end{equation}

However, the computation of $S_L$ and $S_R$ is non-trivial.  To address this, Toro recommends the two-rarefaction approximate in \cite{toro2013riemann}, then Guermond and Popov \cite{guermond2016fast} prove that the two-rarefaction approximated wave speeds indeed provide the correct bounds for Euler equations with $1<\gamma\le 5/3$. 
However, for MHD system, the Riemann problem becomes more complex and is difficult to analyze. In \cite{bouchut2007multiwave, bouchut2010multiwave}, another ``relaxation" approach is used, and the 3-wave and 7-wave approximate Riemann solver are designed, which are proved to be entropy stable. Further, if we simply use the HLL solver \eqref{eq:HLL}, but the wavespeeds $S_L,\ S_R$ are chosen by the above 3-wave solver, then it is also entropy stable \cite{bouchut2010multiwave}. 

Specifically, for two given state $\mathbf U_L,\mathbf U_R$, the explicit formula of $S_L(\mathbf U_L,\mathbf U_R)$ and $S_R(\mathbf U_L,\mathbf U_R)$ along $x$-direction are given by 
$$
S_L=u_L-\mathcal C_L,\quad   S_R=u_R+\mathcal C_R,
$$
where
$$
\mathcal{C} _L=c_{f,L}^{0}+\alpha \left( \left( u_L-u_R \right) _++\frac{\left( p_R-p_L \right) _+}{\rho _Lc_{f,L}+\rho _Rc_{f,R}} \right), 
$$
$$
\mathcal{C} _R=c_{f,R}^{0}+\alpha \left( \left( u_L-u_R \right) _++\frac{\left( p_R-p_L \right) _+}{\rho _Lc_{f,L}+\rho _Rc_{f,R}} \right), 
$$
$$
c_{f,L}^{0}=\left\{ \frac{1}{2}\left( a_L+\frac{\left\| \mathbf{B}_L \right\| ^2}{\rho _Lx_L}+\sqrt{\left( a_L+\frac{\left\| \mathbf{B}_L \right\| ^2}{\rho _Lx_L} \right) ^2-4a_L\frac{B_{x,L}^{2}}{\rho _Lx_L}} \right) \right\} ^{1/2},
$$
$$
c_{f,R}^{0}=\left\{ \frac{1}{2}\left( a_R+\frac{\left\| \mathbf{B}_R \right\| ^2}{\rho _Rx_R}+\sqrt{\left( a_R+\frac{\left\| \mathbf{B}_R \right\| ^2}{\rho _Rx_R} \right) ^2-4a_R\frac{B_{x,R}^{2}}{\rho _Rx_R}} \right) \right\} ^{1/2},
$$and$$
\begin{aligned}
X_L=&\frac{1}{c_{f,L}}\left[ \left( u_L-u_R \right) _++\frac{\left( p_R-p_L \right) _+}{\rho _Lc_{f,L}+\rho _Rc_{f,R}} \right],
\\
X_R=&\frac{1}{c_{f,R}}\left[ \left( u_L-u_R \right) _++\frac{\left( p_R-p_L \right) _+}{\rho _Lc_{f,L}+\rho _Rc_{f,R}} \right], 
\\
x_L=&1-\frac{X_L}{1+\alpha X_L},\quad x_R=1-\frac{X_R}{1+\alpha X_R}
\end{aligned}$$
with $a=\sqrt{\gamma p/\rho},\ \alpha=(\gamma + 1)/2,\ (\cdot)_+=\max\{\cdot,0\}$, and $c_{f,L},c_{f,R}$ denotes the largest eigenvalue of $\partial\mathbf F(\mathbf U)/\partial \mathbf U$ at $\mathbf U=\mathbf U_L,\mathbf U_R$, respectively.

\section{Two-dimensional HLL Riemann solver}\label{app2} 

For four given stages  
at a vertex $\Lambda$, the two-dimensional HLL flux 
$\tilde{E}_z|_{\Lambda}=\tilde{E}_z\left( 
\mathbf{U}_{LD},\mathbf{U}_{LU},\mathbf{U}_{RD},\mathbf{U}_{RU} 
\right) 
$ is calculated by following \cite{chandrashekar2020constraint}. To help with the presentation, we illustrate the notations of states around a vertex $\Lambda$ in Fig \ref{figflux}.

\begin{figure}[htb!]
    \centering
    \includegraphics[width=0.35\linewidth]{figure/fluxnew}
    \caption{The notations around a vertex $\Lambda$.}
     \label{figflux}
\end{figure}

First, the wave speeds are chosen by
$$\begin{aligned}
S_R|_\Lambda&=\max \left\{ S_R\left( \mathbf{U}_{LU},\mathbf{U}_{RU} \right) ,S_R\left( \mathbf{U}_{LD},\mathbf{U}_{RD} \right) \right\} ,
\\S_L|_\Lambda&=\min \left\{ S_L\left( \mathbf{U}_{LU},\mathbf{U}_{RU} \right) ,S_L\left( \mathbf{U}_{LD},\mathbf{U}_{RD}\right)  \right\} ,
\\
S_U|_\Lambda&=\max \left\{ S_R\left( \mathbf{U}_{RD},\mathbf{U}_{RU} \right) ,S_R\left( \mathbf{U}_{LD},\mathbf{U}_{LU} \right) \right\} ,
\\S_D|_\Lambda&=\min \left\{ S_L\left( \mathbf{U}_{RD},\mathbf{U}_{RU} \right) ,S_R\left( \mathbf{U}_{LD},\mathbf{U}_{LU} \right) \right\}\end{aligned}
$$
to match the wave speeds of the nodal DG scheme 
in the cell. Denote $$\mathcal S_R=\max\{S_R,0\},\quad \mathcal S_U=\max\{S_U,0\}, \quad \mathcal S_L=\min\{S_L,0\},\quad  \mathcal S_D=\min\{S_D,0\},$$
then the value of $\tilde E_z$ is given by
$$\begin{aligned}
\tilde E_z^{HLL}&=\frac{1}{4}\left( E_{z}^{*,R}+E_{z}^{*,L}+E_{z}^{*,U}+E_{z}^{*,D} \right) 
\\
&\quad -\frac{1}{4}\mathcal{S} _U\left( B_{x}^{U,*}-B_{x}^{**} \right) -\frac{1}{4}\mathcal{S} _D\left( B_{x}^{D,*}-B_{x}^{**} \right) 
\\
&\quad +\frac{1}{4}\mathcal{S} _R\left( B_{y}^{R,*}-B_{y}^{**} \right) +\frac{1}{4}\mathcal{S} _L\left( B_{y}^{L,*}-B_{y}^{**} \right), 
\end{aligned}
$$
where
$$
E_{z}^{*,R}=\mathbf{\hat{G}}_{6}^{HLL}\left( \mathbf{U}_{RD},\mathbf{U}_{RU} \right) , \quad 
E_{z}^{*,L}=\mathbf{\hat{G}}_{6}^{HLL}\left( \mathbf{U}_{LD},\mathbf{U}_{LU} \right), 
$$
$$
E_{z}^{*,U}=-\mathbf{\hat{F}}_{7}^{HLL}\left( \mathbf{U}_{LU},\mathbf{U}_{RU} \right) , \quad 
E_{z}^{*,D}=-\mathbf{\hat{F}}_{7}^{HLL}\left( \mathbf{U}_{LD},\mathbf{U}_{RD} \right), 
$$
and
$$\begin{aligned}
B_{x}^{**}=\frac{1}{2\Delta \mathcal S}&\left[ 
	2\mathcal{S} _R\mathcal{S} _UB_{x}^{RU}-2\mathcal{S} _L\mathcal{S} _UB_{x}^{LU}-2\mathcal{S} _R\mathcal{S} _DB_{x}^{RD}+2\mathcal{S} _L\mathcal{S} _DB_{x}^{LD}\right.
 \\ &-\mathcal{S} _R\left( E_{z}^{RU}-E_{z}^{RD} \right) +\mathcal{S} _L\left( E_{z}^{LU}-E_{z}^{LD} \right) 
 \\ &\left.-\left( \mathcal{S} _R-\mathcal{S} _L \right) \left( E_{z}^{*,U}-E_{z}^{*,D} \right) \right], 
 \end{aligned}
$$
$$\begin{aligned}
B_{y}^{**}=\frac{1}{2\Delta\mathcal S}&\left[ 
	2\mathcal{S} _R\mathcal{S} _UB_{y}^{RU}-2\mathcal{S} _L\mathcal{S} _UB_{y}^{LU}-2\mathcal{S} _R\mathcal{S} _DB_{y}^{RD}+2\mathcal{S} _L\mathcal{S} _DB_{y}^{LD}\right.\\
	&+\mathcal{S} _U\left( E_{z}^{RU}-E_{z}^{LU} \right) -\mathcal{S} _D\left( E_{z}^{RD}-E_{z}^{LD} \right)\\
	&\left.+\left( \mathcal{S} _U-\mathcal{S} _D \right) \left( E_{z}^{*,R}-E_{z}^{*,L} \right) \right], \end{aligned}
$$
where $\Delta \mathcal S=(\mathcal S_R-\mathcal S_L)(\mathcal S_U-\mathcal S_D)$.

\section{The reconstruction for small $k$}\label{app4} We give a brief discussion about the LS reconstruction problem in Section 3.3 for small $k$. We rewrite the linear system (3.18) as
$$
\mathbf{G}\left[ \begin{array}{c}
	\mathbf{B}^{rec}\\
	\boldsymbol{\lambda }\\
\end{array} \right] =\left[ \begin{array}{c}
	M_2\mathbf{\tilde{\mathbf B}}\\
	\mathbf{b}_1\\
\end{array} \right], 
$$
then $\mathbf G^{-1}$ can be given by
$$
\mathbf{G}^{-1}=\left[ \begin{matrix}
	M^{-1}-M^{-1}A_1^T\mathbf{S}A_1M^{-1}&		M^{-1}A_1^T\mathbf{S}\\
	-\mathbf{S}A_1M^{-1}&		\mathbf{S}\\
\end{matrix} \right], 
$$
where $\mathbf S=(A_1MA_1^T)^{-1}$ is the Schur complement of $M$. In the following, we will assume $\Delta x=\Delta y$.

To help understand, we first consider the simplest case $k=0$, and the 2 points Gauss-Lobatto quadrature is used. Now we have
$$
M=\left[ \begin{matrix}
	1&		0\\
	0&		1\\
\end{matrix} \right] =I,\quad D=\left[ \begin{matrix}
	0.5&		-0.5\\
	0.5&		-0.5\\
\end{matrix} \right]. 
$$
Assume $$ b_x^+ = a_0^+,\quad b_x^- = a_0^-,\quad b_y^+ = b_0^+,\quad b_y^- = b_0^-. $$
Then, the original linear system of reconstruction (3.16) is
\begin{equation}\label{eq:P0-1}
\left[ \begin{matrix}
	-1&		1&		0&		0&		-1&		0&		1&		0\\
	-1&		1&		0&		0&		0&		-1&		0&		1\\
	0&		0&		-1&		1&		-1&		0&		1&		0\\
	0&		0&		-1&		1&		0&		-1&		0&		1\\
	0&		1&		0&		0&		0&		0&		0&		0\\
	0&		0&		0&		1&		0&		0&		0&		0\\
	1&		0&		0&		0&		0&		0&		0&		0\\
	0&		0&		1&		0&		0&		0&		0&		0\\
	0&		0&		0&		0&		0&		0&		1&		0\\
	0&		0&		0&		0&		0&		0&		0&		1\\
	0&		0&		0&		0&		1&		0&		0&		0\\
	0&		0&		0&		0&		0&		1&		0&		0\\
\end{matrix} \right] \left[ \begin{matrix}
	B_{x,00}\\
	B_{x,10}\\
	B_{x,01}\\
	B_{x,11}\\
	B_{y,00}\\
	B_{y,10}\\
	B_{y,01}\\
	B_{y,11}\\
\end{matrix} \right] =\left[ \begin{matrix}
	0\\
	0\\
	0\\
	0\\
	a_{0}^{+}\\
	a_{0}^{+}\\
	a_{0}^{-}\\
	a_{0}^{-}\\
	b_{0}^{+}\\
	b_{0}^{+}\\
	b_{0}^{-}\\
	b_{0}^{-}\\
\end{matrix} \right],
\end{equation}
which is a $12\times 8$ linear system. To simplify the form, we have multiplied a factor 2 for the first four rows. It is notable that the last 8 rows of $A$ already form a full rank $8\times 8$ matrix, hence the system \eqref{eq:P0-1} has at most one solution. Since the number of equations is larger than DOFs, it seems that there may have ``\,$0 = d$\," rows with $d\ne 0$ in the simplified stepped system, which will lead to the system non-solvable. However, applying some elementary row operations to $A$ yields

$$
\left[ \begin{matrix}
	0&		0&		0&		0&		0&		0&		0&		0\\
	0&		0&		0&		0&		0&		0&		0&		0\\
	0&		0&		0&		0&		0&		0&		0&		0\\
	0&		0&		0&		0&		0&		0&		0&		0\\
	0&		1&		0&		0&		0&		0&		0&		0\\
	0&		0&		0&		1&		0&		0&		0&		0\\
	1&		0&		0&		0&		0&		0&		0&		0\\
	0&		0&		1&		0&		0&		0&		0&		0\\
	0&		0&		0&		0&		0&		0&		1&		0\\
	0&		0&		0&		0&		0&		0&		0&		1\\
	0&		0&		0&		0&		1&		0&		0&		0\\
	0&		0&		0&		0&		0&		1&		0&		0\\
\end{matrix} \right] \left[ \begin{matrix}
	B_{x,00}\\
	B_{x,10}\\
	B_{x,01}\\
	B_{x,11}\\
	B_{y,00}\\
	B_{y,10}\\
	B_{y,01}\\
	B_{y,11}\\
\end{matrix} \right] =\left[ \begin{matrix}
	a_{0}^{-}-a_{0}^{+}+b_{0}^{-}-b_{0}^{+}\\
	a_{0}^{-}-a_{0}^{+}+b_{0}^{-}-b_{0}^{+}\\
	a_{0}^{-}-a_{0}^{+}+b_{0}^{-}-b_{0}^{+}\\
	a_{0}^{-}-a_{0}^{+}+b_{0}^{-}-b_{0}^{+}\\
	a_{0}^{+}\\
	a_{0}^{+}\\
	a_{0}^{-}\\
	a_{0}^{-}\\
	b_{0}^{+}\\
	b_{0}^{+}\\
	b_{0}^{-}\\
	b_{0}^{-}\\
\end{matrix} \right]. 
$$
Hence, the system is solvable if and only if the cell-average constraint is satisfied, which indicates that $$a_0^+-a_0^-+b_0^+-b_0^-=0.$$
Then, the unique solution of \eqref{eq:P0-1} is
\begin{equation}\begin{aligned}\label{eq:P0-solution}
B_{x,00}=B_{x,01}=a_{0}^{-},&\quad B_{x,10}=B_{x,11}=a_{0}^{+},
\\
B_{y,00}=B_{y,10}=b_{0}^{-},&\quad B_{y,01}=B_{y,11}=b_{0}^{+}.
\end{aligned}
\end{equation}
On the other hand, if we directly consider the system (3.18), then we can see $A_1$ is a $8\times 8$ full rank matrix. Since $M=I$, we can derive that $\mathbf S=(A_1^{T})^{-1}A_1^{-1}$, and
$$
\mathbf{G}^{-1}=\left[ \begin{matrix}
	O&		A_1^{-1}\\
	-\left( A_1^T \right) ^{-1}&		(A_1^T)^{-1}A_1^{-1}\\
\end{matrix} \right]. 
$$
Therefore, we have
$$
\left[ \begin{array}{c}
	\mathbf{B}^{rec}\\
	\mathbf{\lambda }\\
\end{array} \right] =\left[ \begin{matrix}
	O&		A_1^{-1}\\
	-\left( A_1^T \right) ^{-1}&		(A_1^T)^{-1}A_1^{-1}\\
\end{matrix} \right] \left[ \begin{array}{c}
	\mathbf{B}^{\mathrm{DG}}\\
	\mathbf{b}_1\\
\end{array} \right], 
$$
so $\mathbf B^{rec}= A_1^{-1}\mathbf b_1$, it is also the solution of $A\mathbf B=\mathbf b$, thus we recover \eqref{eq:P0-solution}. This is also consistent with the conclusion in \cite{balsara2021globally}.

However, for $k> 0$, the system has become very complicated.  When $k=1$, the size of $A$ is a $21\times 18$, and the size of $\mathbf G$ is $35\times 35$. For $k=2$, the sizes are respectively $32\times 32$ and $60\times 60$. For $k=3$, the sizes are respectively $ 45\times 50 $ and $91\times 91$. Therefore, it is difficult to study the underlying mechanism or give the explicit formulation like \eqref{eq:P0-solution} for the reconstruction equation with general $k$. In Fig \ref{figmat}, we present the structure of nonzero elements in $\mathbf G^{-1}$ for $k=1,2,3$ as a reference. 

\begin{figure}[htbp!]
    \centering
    \subfigure[$k=1$.]{
        \includegraphics[width=0.31\linewidth]{figure/P1rec}}
    \subfigure[$k=2$.]{
        \includegraphics[width=0.31\linewidth]{figure/P2rec}}
    \subfigure[$k=3$.]{
        \includegraphics[width=0.31\linewidth]{figure/P3rec}}
    \caption{The structure of nonzero elements in $\mathbf G^{-1}$. }
    \label{figmat}
\end{figure}

In addition, we give the full express of $\mathbf G^{-1}$ for $k=1$. The first 5 columns of $\mathbf G^{-1}$ are\newpage 
 $$\left[ \begin{matrix} 
 0 &0 &0 &0 &0 \\ 
0 &9/16 &0 &0 &0 \\ 
0 &0 &0 &0 &0 \\ 
0 &0 &0 &0 &0 \\ 
0 &0 &0 &0 &0 \\ 
0 &0 &0 &0 &0 \\ 
0 &0 &0 &0 &0 \\ 
0 &-9/16 &0 &0 &0 \\ 
0 &0 &0 &0 &0 \\ 
0 &0 &0 &0 &0 \\ 
0 &0 &0 &0 &0 \\ 
0 &0 &0 &0 &0 \\ 
0 &-9/16 &0 &0 &0 \\ 
0 &0 &0 &0 &0 \\ 
0 &9/16 &0 &0 &0 \\ 
0 &0 &0 &0 &0 \\ 
0 &0 &0 &0 &0 \\ 
0 &0 &0 &0 &0 \\ 
446/10487 &-361/4426 &446/10487 &0 &0 \\ 
0 &-407/5879 &1345/18033 &686/18395 &-407/5879 \\ 
194/2497 &-811/8786 &158/7263 &2699/54280 &-811/8786 \\ 
-293/5856 &482/5241 &-293/5856 &293/2928 &-403/2191 \\ 
31/13608 &-236/56361 &31/13608 &-31/6804 &225/26867 \\ 
-195/1351 &0 &195/1351 &-195/1351 &0 \\ 
1262/6927 &0 &-1262/6927 &-1217/3340 &0 \\ 
5143/432011 &0 &-5143/432011 &-10286/432011 &0 \\ 
-3599/5453 &0 &937/6487 &-115/589 &0 \\ 
0 &0 &-137/1263 &2539/11975 &0 \\ 
0 &0 &336/1285 &609/3007 &0 \\ 
-99/90076 &0 &-1471/2543 &513/7487 &0 \\ 
-338/963 &-265/724 &-338/963 &0 &0 \\ 
152/7003 &181/7664 &152/7003 &-304/7003 &-181/3832 \\ 
-883/3115 &-223/723 &-883/3115 &847/1494 &446/723 \\ 
89/1024 &884/2323 &213/499 &737/2869 &884/2323 \\ 
-413/985 &-469/1397 &-203/5977 &-526/2321 &-469/1397 \\ 
 \end{matrix} \right]. $$ 

\newpage
Column 6 to 10 of $\mathbf G^{-1}$ are
  $$\left[ \begin{matrix} 
 0 &0 &0 &0 &0 \\ 
0 &0 &-9/16 &0 &0 \\ 
0 &0 &0 &0 &0 \\ 
0 &0 &0 &0 &0 \\ 
0 &0 &0 &0 &0 \\ 
0 &0 &0 &0 &0 \\ 
0 &0 &0 &0 &0 \\ 
0 &0 &9/16 &0 &0 \\ 
0 &0 &0 &0 &0 \\ 
0 &0 &0 &0 &0 \\ 
0 &0 &0 &0 &0 \\ 
0 &0 &0 &0 &0 \\ 
0 &0 &9/16 &0 &0 \\ 
0 &0 &0 &0 &0 \\ 
0 &0 &-9/16 &0 &0 \\ 
0 &0 &0 &0 &0 \\ 
0 &0 &0 &0 &0 \\ 
0 &0 &0 &0 &0 \\ 
0 &-446/10487 &361/4426 &-446/10487 &446/10487 \\ 
686/18395 &1345/18033 &-407/5879 &0 &-158/7263 \\ 
2699/54280 &158/7263 &-811/8786 &194/2497 &1345/18033 \\ 
293/2928 &-293/5856 &482/5241 &-293/5856 &-31/13608 \\ 
-31/6804 &31/13608 &-236/56361 &31/13608 &-293/5856 \\ 
195/1351 &-195/1351 &0 &195/1351 &-195/1351 \\ 
1217/3340 &1262/6927 &0 &-1262/6927 &-5143/432011 \\ 
10286/432011 &5143/432011 &0 &-5143/432011 &1262/6927 \\ 
51/881 &739/2742 &0 &-96/3349 &491/831 \\ 
723/6241 &5078/11975 &0 &946/2781 &-1395/8672 \\ 
-162/1069 &625/1543 &0 &-2033/3601 &-341/1901 \\ 
-809/2711 &255/1846 &0 &-77/4190 &524/3107 \\ 
0 &338/963 &265/724 &338/963 &-338/963 \\ 
-304/7003 &152/7003 &181/7664 &152/7003 &-883/3115 \\ 
847/1494 &-883/3115 &-223/723 &-883/3115 &-152/7003 \\ 
737/2869 &213/499 &884/2323 &89/1024 &-203/5977 \\ 
-526/2321 &-203/5977 &-469/1397 &-413/985 &-213/499 \\ 
 \end{matrix} \right]. $$ 

\newpage

Column 11 to 15 of $\mathbf G^{-1}$ are
 $$\left[ \begin{matrix} 
 0 &0 &0 &0 &0 \\ 
0 &0 &-9/16 &0 &9/16 \\ 
0 &0 &0 &0 &0 \\ 
0 &0 &0 &0 &0 \\ 
0 &0 &0 &0 &0 \\ 
0 &0 &0 &0 &0 \\ 
0 &0 &0 &0 &0 \\ 
0 &0 &9/16 &0 &-9/16 \\ 
0 &0 &0 &0 &0 \\ 
0 &0 &0 &0 &0 \\ 
0 &0 &0 &0 &0 \\ 
0 &0 &0 &0 &0 \\ 
0 &0 &9/16 &0 &-9/16 \\ 
0 &0 &0 &0 &0 \\ 
0 &0 &-9/16 &0 &9/16 \\ 
0 &0 &0 &0 &0 \\ 
0 &0 &0 &0 &0 \\ 
0 &0 &0 &0 &0 \\ 
0 &-446/10487 &-361/4426 &0 &361/4426 \\ 
-2699/54280 &-194/2497 &811/8786 &811/8786 &811/8786 \\ 
686/18395 &0 &-407/5879 &-407/5879 &-407/5879 \\ 
31/6804 &-31/13608 &236/56361 &-225/26867 &236/56361 \\ 
293/2928 &-293/5856 &482/5241 &-403/2191 &482/5241 \\ 
-195/1351 &-195/1351 &0 &0 &0 \\ 
10286/432011 &-5143/432011 &0 &0 &0 \\ 
-1217/3340 &1262/6927 &0 &0 &0 \\ 
551/2084 &-169/2723 &0 &0 &0 \\ 
-823/16086 &301/5142 &0 &0 &0 \\ 
-3234/139709 &461/3464 &0 &0 &0 \\ 
-572/2423 &-1841/2873 &0 &0 &0 \\ 
0 &338/963 &-265/724 &0 &265/724 \\ 
847/1494 &-883/3115 &-223/723 &446/723 &-223/723 \\ 
304/7003 &-152/7003 &-181/7664 &181/3832 &-181/7664 \\ 
-526/2321 &-413/985 &-469/1397 &-469/1397 &-469/1397 \\ 
-737/2869 &-89/1024 &-884/2323 &-884/2323 &-884/2323 \\ 
 \end{matrix} \right]. $$ 

\newpage
Column 16 to 20 of $G^{-1}$ are
 $$\left[ \begin{matrix} 
 0 &0 &0 &446/10487 &0 \\ 
0 &0 &0 &-361/4426 &-407/5879 \\ 
0 &0 &0 &446/10487 &1345/18033 \\ 
0 &0 &0 &0 &686/18395 \\ 
0 &0 &0 &0 &-407/5879 \\ 
0 &0 &0 &0 &686/18395 \\ 
0 &0 &0 &-446/10487 &1345/18033 \\ 
0 &0 &0 &361/4426 &-407/5879 \\ 
0 &0 &0 &-446/10487 &0 \\ 
0 &0 &0 &446/10487 &-158/7263 \\ 
0 &0 &0 &0 &-2699/54280 \\ 
0 &0 &0 &-446/10487 &-194/2497 \\ 
0 &0 &0 &-361/4426 &811/8786 \\ 
0 &0 &0 &0 &811/8786 \\ 
0 &0 &0 &361/4426 &811/8786 \\ 
0 &0 &0 &446/10487 &-194/2497 \\ 
0 &0 &0 &0 &-2699/54280 \\ 
0 &0 &0 &-446/10487 &-158/7263 \\ 
446/10487 &0 &-446/10487 &-23/1712 &0 \\ 
-194/2497 &-2699/54280 &-158/7263 &0 &-287/6896 \\ 
0 &686/18395 &1345/18033 &0 &0 \\ 
-31/13608 &31/6804 &-31/13608 &0 &-94/5141 \\ 
-293/5856 &293/2928 &-293/5856 &0 &199/7414 \\ 
195/1351 &195/1351 &195/1351 &0 &0 \\ 
5143/432011 &-10286/432011 &5143/432011 &0 &0 \\ 
-1262/6927 &1217/3340 &-1262/6927 &0 &0 \\ 
1022/16221 &31/2753 &-251/6200 &0 &67/10675 \\ 
357/604 &401/8908 &-731/1459 &0 &-27/6463 \\ 
646/2335 &961/2904 &3219/8357 &0 &63/14102 \\ 
222/2929 &120/917 &3951/21250 &0 &56/50269 \\ 
-338/963 &0 &338/963 &-90/2261 &0 \\ 
-883/3115 &847/1494 &-883/3115 &0 &-65/1076 \\ 
-152/7003 &304/7003 &-152/7003 &0 &144/3743 \\ 
-413/985 &-526/2321 &-203/5977 &0 &199/1660 \\ 
-89/1024 &-737/2869 &-213/499 &0 &62/2495 \\ 
 \end{matrix} \right]. $$ 

 \newpage
 The 21 to 25 columns of $\mathbf G^{-1}$ are
  $$\left[ \begin{matrix} 
 0 &0 &0 &446/10487 &0 \\ 
0 &0 &0 &-361/4426 &-407/5879 \\ 
0 &0 &0 &446/10487 &1345/18033 \\ 
0 &0 &0 &0 &686/18395 \\ 
0 &0 &0 &0 &-407/5879 \\ 
0 &0 &0 &0 &686/18395 \\ 
0 &0 &0 &-446/10487 &1345/18033 \\ 
0 &0 &0 &361/4426 &-407/5879 \\ 
0 &0 &0 &-446/10487 &0 \\ 
0 &0 &0 &446/10487 &-158/7263 \\ 
0 &0 &0 &0 &-2699/54280 \\ 
0 &0 &0 &-446/10487 &-194/2497 \\ 
0 &0 &0 &-361/4426 &811/8786 \\ 
0 &0 &0 &0 &811/8786 \\ 
0 &0 &0 &361/4426 &811/8786 \\ 
0 &0 &0 &446/10487 &-194/2497 \\ 
0 &0 &0 &0 &-2699/54280 \\ 
0 &0 &0 &-446/10487 &-158/7263 \\ 
446/10487 &0 &-446/10487 &-23/1712 &0 \\ 
-194/2497 &-2699/54280 &-158/7263 &0 &-287/6896 \\ 
0 &686/18395 &1345/18033 &0 &0 \\ 
-31/13608 &31/6804 &-31/13608 &0 &-94/5141 \\ 
-293/5856 &293/2928 &-293/5856 &0 &199/7414 \\ 
195/1351 &195/1351 &195/1351 &0 &0 \\ 
5143/432011 &-10286/432011 &5143/432011 &0 &0 \\ 
-1262/6927 &1217/3340 &-1262/6927 &0 &0 \\ 
1022/16221 &31/2753 &-251/6200 &0 &67/10675 \\ 
357/604 &401/8908 &-731/1459 &0 &-27/6463 \\ 
646/2335 &961/2904 &3219/8357 &0 &63/14102 \\ 
222/2929 &120/917 &3951/21250 &0 &56/50269 \\ 
-338/963 &0 &338/963 &-90/2261 &0 \\ 
-883/3115 &847/1494 &-883/3115 &0 &-65/1076 \\ 
-152/7003 &304/7003 &-152/7003 &0 &144/3743 \\ 
-413/985 &-526/2321 &-203/5977 &0 &199/1660 \\ 
-89/1024 &-737/2869 &-213/499 &0 &62/2495 \\ 
 \end{matrix} \right]. $$ 

 \newpage
Column 26 to 30 of $\mathbf G^{-1}$ are
 $$\left[ \begin{matrix} 
 5143/432011 &-3599/5453 &0 &0 &-99/90076 \\ 
0 &0 &0 &0 &0 \\ 
-5143/432011 &937/6487 &-137/1263 &336/1285 &-1471/2543 \\ 
-10286/432011 &-115/589 &2539/11975 &609/3007 &513/7487 \\ 
0 &0 &0 &0 &0 \\ 
10286/432011 &51/881 &723/6241 &-162/1069 &-809/2711 \\ 
5143/432011 &739/2742 &5078/11975 &625/1543 &255/1846 \\ 
0 &0 &0 &0 &0 \\ 
-5143/432011 &-96/3349 &946/2781 &-2033/3601 &-77/4190 \\ 
1262/6927 &491/831 &-1395/8672 &-341/1901 &524/3107 \\ 
-1217/3340 &551/2084 &-823/16086 &-3234/139709 &-572/2423 \\ 
1262/6927 &-169/2723 &301/5142 &461/3464 &-1841/2873 \\ 
0 &0 &0 &0 &0 \\ 
0 &0 &0 &0 &0 \\ 
0 &0 &0 &0 &0 \\ 
-1262/6927 &1022/16221 &357/604 &646/2335 &222/2929 \\ 
1217/3340 &31/2753 &401/8908 &961/2904 &120/917 \\ 
-1262/6927 &-251/6200 &-731/1459 &3219/8357 &3951/21250 \\ 
0 &0 &0 &0 &0 \\ 
0 &67/10675 &-27/6463 &63/14102 &56/50269 \\ 
0 &-74/64347 &-111/20717 &-45/9634 &95/18561 \\ 
0 &53/12731 &-68/6223 &-45/20756 &152/19417 \\ 
0 &-90/9571 &21/29873 &-61/5987 &37/11708 \\ 
-149/3989 &0 &0 &0 &0 \\ 
0 &-49/1496 &110/8839 &81/1768 &145/3054 \\ 
-2/15 &429/14929 &-61/5587 &-91/2264 &-142/3409 \\ 
429/14929 &-797/5375 &107/6728 &56/3313 &182/5961 \\ 
-61/5587 &107/6728 &-297/2248 &-112/8103 &8/11573 \\ 
-91/2264 &56/3313 &-112/8103 &-425/2513 &-175/4867 \\ 
-142/3409 &182/5961 &8/11573 &-175/4867 &-1250/7501 \\ 
0 &0 &0 &0 &0 \\ 
0 &-332/6139 &59/9990 &-285/4963 &92/5557 \\ 
0 &131/5963 &-80/1293 &-155/11002 &277/6160 \\ 
0 &106/3253 &-178/6237 &87/4607 &179/15250 \\ 
0 &632/47779 &239/9859 &216/7151 &-429/16265 \\ 
 \end{matrix} \right]. $$

 \newpage
Column 31 to 35 of $\mathbf G^{-1}$ are
  $$\left[ \begin{matrix} 
 -338/963 &152/7003 &-883/3115 &89/1024 &-413/985 \\ 
-265/724 &181/7664 &-223/723 &884/2323 &-469/1397 \\ 
-338/963 &152/7003 &-883/3115 &213/499 &-203/5977 \\ 
0 &-304/7003 &847/1494 &737/2869 &-526/2321 \\ 
0 &-181/3832 &446/723 &884/2323 &-469/1397 \\ 
0 &-304/7003 &847/1494 &737/2869 &-526/2321 \\ 
338/963 &152/7003 &-883/3115 &213/499 &-203/5977 \\ 
265/724 &181/7664 &-223/723 &884/2323 &-469/1397 \\ 
338/963 &152/7003 &-883/3115 &89/1024 &-413/985 \\ 
-338/963 &-883/3115 &-152/7003 &-203/5977 &-213/499 \\ 
0 &847/1494 &304/7003 &-526/2321 &-737/2869 \\ 
338/963 &-883/3115 &-152/7003 &-413/985 &-89/1024 \\ 
-265/724 &-223/723 &-181/7664 &-469/1397 &-884/2323 \\ 
0 &446/723 &181/3832 &-469/1397 &-884/2323 \\ 
265/724 &-223/723 &-181/7664 &-469/1397 &-884/2323 \\ 
-338/963 &-883/3115 &-152/7003 &-413/985 &-89/1024 \\ 
0 &847/1494 &304/7003 &-526/2321 &-737/2869 \\ 
338/963 &-883/3115 &-152/7003 &-203/5977 &-213/499 \\ 
-90/2261 &0 &0 &0 &0 \\ 
0 &-65/1076 &144/3743 &199/1660 &62/2495 \\ 
0 &144/3743 &65/1076 &62/2495 &-199/1660 \\ 
0 &-17/3218 &573/3355 &298/4075 &-217/3070 \\ 
0 &573/3355 &17/3218 &-217/3070 &-298/4075 \\ 
0 &0 &0 &0 &0 \\ 
0 &0 &0 &0 &0 \\ 
0 &0 &0 &0 &0 \\ 
0 &-332/6139 &131/5963 &106/3253 &632/47779 \\ 
0 &59/9990 &-80/1293 &-178/6237 &239/9859 \\ 
0 &-285/4963 &-155/11002 &87/4607 &216/7151 \\ 
0 &92/5557 &277/6160 &179/15250 &-429/16265 \\ 
-202/581 &0 &0 &0 &0 \\ 
0 &-1189/1092 &0 &473/1203 &356/931 \\ 
0 &0 &-1189/1092 &-356/931 &473/1203 \\ 
0 &473/1203 &-356/931 &-1321/1514 &0 \\ 
0 &356/931 &473/1203 &0 &-1321/1514 \\ 
 \end{matrix} \right]. $$

\bibliographystyle{siamplain}
\bibliography{references}

\end{document}
